# Supplementary material for: Giant Collective Spin-Orbit Field in a Quantum Well: Fine Structure of Spin Plasmons
Source: arXiv:1310.7508 ancillary file (2013-10-28)
Supplement: Supplementary file 1 [file Supplemental_Material.pdf]

# Supplemental Material for:

# Giant Collective Spin-Orbit Field in a Quantum Well: Fine Structure of Spin Plasmons

F. Baboux,[1,*] F. Perez,[1] C. A. Ullrich,[2] I. D'Amico,[3] J. Gómez,[1,†] and M. Bernard[1]

[1] *Institut des Nanosciences de Paris, CNRS/Université Paris VI, Paris 75005, France*

[2] *Department of Physics and Astronomy, University of Missouri, Columbia, Missouri 65211, USA*

[3] *Department of Physics, University of York, York YO10 5DD, United Kingdom*

## EXPERIMENT

The studied sample is an asymmetrically modulation-doped GaAs/$Al_{0.3}Ga_{0.7}As$ quantum well, grown along the [001] direction by molecular beam epitaxy. The 200 Å-thick well was doped with two Si delta layers, separated from the well by spacer thicknesses of 350 and 400 Å respectively. The electron density is $2.3 \times 10^{11}$ cm$^{-2}$, and the mobility $2 \times 10^7$ cm$^2$ V$^{-1}$ s$^{-1}$ at the working temperature $T \simeq 2$ K (superfluid helium), as determined from Hall measurements.

The inelastic light scattering setup, depicted in Fig. 2(a) of the Letter, is in the backscattering geometry. The average angle $\theta$ of the incoming and backscattered light with respect to the normal direction can be changed to transfer a Raman momentum $\mathbf{q}$ of amplitude $q = \frac{4\pi}{\lambda} \cos\frac{\gamma}{2} \sin\theta$, with $\gamma \simeq 3°$ and $\lambda \simeq 770$ nm the exciting wavelength.

Measurements are performed in an pumped-helium optical cryostat embedding a superconducting coil. The scattered light is dispersed by a Dilor XY triple Raman spectrometer in additive mode.

To deconvolute the linewidth $w$ of the composite Raman peak observed (Fig. 2(a) of the Letter), we fit the sum of two identical Lorentzian peaks of linewidth $\Gamma$ separated by $\delta$, with a single Lorentzian, yielding a linewidth $w$. We then numerically invert the $w(\delta)$ plot to obtain the $\delta(w)$ function.

## CALCULATION OF INTERSUBBAND SPIN PLASMON DISPERSIONS

The formal framework for calculating intersubband spin plasmon dispersions in quantum wells, in the presence of spin-orbit coupling, is based on time-dependent density-functional theory within the effective-mass approximation, as described in detail in Refs. [1, 2]. We have here extended this formalism to account for external in-plane magnetic fields. The calculation proceeds in two steps. First, the two-component spinor subband envelope functions $\psi_j(\mathbf{k}, z)$ are calculated via

$$\sum_{\beta=\uparrow,\downarrow} \left[ \hat{h}\delta_{\alpha\beta} + v^{\rm xc}_{\alpha\beta} + \frac{g\mu_{\rm B}}{2} [\vec{\sigma} \cdot (\mathbf{B}_{\rm ext} + \mathbf{B}_{\rm SO}(\mathbf{k}))]_{\alpha\beta} \right] \psi_{j\beta} = \varepsilon_j \psi_{j\alpha} \,, \tag{1}$$

where $\hat{h}$ is the single-particle kinetic energy operator plus quantum well confining potential and Hartree potential, $v^{\rm xc}_{\alpha\beta}$ is the spin-dependent exchange-correlation (xc) potential in local-density approximation, and $\vec{\sigma}$ is the vector of Pauli matrices. The parameters of our modulation-doped GaAs quantum well are taken as input.

The second step is to calculate the intersubband spin plasmon dispersions using linear-response theory. Formally, the plasmon excitation energies are obtained from the poles of the response function

$$\Pi = \frac{\Pi_0}{1 - \Pi_0 F^{\rm Hxc}} \,, \tag{2}$$

where $\Pi_0$ is the noninteracting response function, built from the solutions of Eq. (1), which determines the single-particle excitation spectrum. $\Pi_0$ and $\Pi$ are represented as $4 \times 4$ matrices, describing the charge-density response and three components of the magnetization response. The formation of collective plasmon excitations is a consequence of dynamical many-body effects (Hartree and xc), accounted for via $F^{\rm Hxc}$. The spin plasmons arise solely from the xc part of $F^{\rm Hxc}$, which is treated in an adiabatic local-density approximation [1, 2].

Based on the given quantum well parameters, the Rashba and Dresselhaus constants for the $n$th subband, $\alpha_n$ and $\beta_n$, can be calculated using $\mathbf{k}\cdot\mathbf{p}$ theory [3, 4]. For the Dresselhaus parameter for bulk GaAs we instead use a recent result from an ab-initio GW calculation [5], $\gamma^{\rm GW}_{\rm GaAs} = 6.4$ eV Å$^3$, which is about 4 times smaller than the $\mathbf{k}\cdot\mathbf{p}$ value. We thus obtain $\alpha_1^{\rm kp} = 0.84$ meV Å, $\alpha_2^{\rm kp} = 0.66$ meV Å and $\beta_1^{\rm GW} = 0.93$ meV Å, $\beta_2^{\rm GW} = 3.3$ meV Å. However, to reproduce the experimental data in Figs. 2(b)–(d) and 4 of the Letter, we found it necessary to rescale the values of the Rashba and Dresselhaus constants by 4.2 and 0.24, respectively, i.e., to use $\alpha_{1,2} = 4.2\alpha^{\rm kp}_{1,2}$ and $\beta_{1,2} = 0.24\beta^{\rm GW}_{1,2}$.

We emphasize that these are the only fitting parameters of our theory. Note that $\sqrt{\overline{\alpha}^2 + \overline{\beta}^2} \simeq 1.4 \times \sqrt{\overline{\alpha^{\mathrm{kp}}}^2 + \overline{\beta^{\mathrm{GW}}}^2}$. Thus, the enhancement factor from single-particle to collective spin-orbit magnetic field, which is found of 5.25 with the fitted values for $\alpha$ and $\beta$, would be close to 7.3 with the predicted ones.

## CALCULATION OF THE SPIN COULOMB DRAG LINEWIDTH

The spin Coulomb drag linewidth $\Gamma_{\mathrm{SCD}}$ is calculated within the framework of time-dependent spin-current density-functional theory, with dissipative effects (SCD and viscosity) included from first principles, see Ref. [6]. The SCD enters the formulation as one of the contributions to the exchange-correlation kernel. This contribution is calculated within a three-dimensional local-density approximation, which accounts for inhomogeneity in the growth direction.

Improving over Ref. [6], we now accurately model the first-subband envelope function using a density-functional scheme, with the parameters of the experimental quantum well (doping density, quantum well width, doping-layer position) as input. As the SCD linewidth may be very sensitive to the envelope function shape, the uncertainty of these input parameters is important. For the sample considered, reasonable uncertainties over the experimental parameters produce a SCD linewidth variation of about 15%. We have also derived the finite-$q$ correction to $\Gamma_{\mathrm{SCD}}$, which is only second order in $q$. In contrast with Ref. [6], we have included in the current calculations the dissipative effects stemming from the viscosity term of the exchange-correlation kernel. In principle, this contribution might be substantial as the quantum well is strongly asymmetric, but it turns out to be one order of magnitude smaller than the SCD contribution. This confirms the latter to be the largest source of intrinsic dissipation for an ISB spin plasmon.

For the studied sample we find $\Gamma_{\mathrm{SCD}} \simeq 0.4$ meV, which overestimates the linewidth. We find a quantitatively similar overestimate when calculating the spin plasmon linewidth of the experimental results in Ref. [7]. In the case of charge plasmons in quantum wells it was argued [8] that the three-dimensional local-density approximation does not account properly for the subband quantization, which acts as a bottleneck for energy-momentum dissipation from the collective to the in-plane degrees of freedom. Hence, it is not surprising that our theoretical estimate for $\Gamma_{\mathrm{SCD}}$ lies above the experimental linewidth while still providing the correct order of magnitude.

There are no adjustable parameters in the theory.

---

* Corresponding author: florent.baboux@insp.upmc.fr
† Present address: Centro Atómico Bariloche, Bariloche, Argentina.
[1] C. A. Ullrich and M. E. Flatté, Phys. Rev. B **66**, 205305 (2002).
[2] C. A. Ullrich and M. E. Flatté, Phys. Rev. B **68**, 235310 (2003).
[3] P. Pfeffer and W. Zawadzki, Phys. Rev. B **59**, 5312(R) (1999).
[4] R. Winkler, *Spin-Orbit Coupling Effects in Two-Dimensional Electron and Hole Systems* (Springer, Berlin, 2003).
[5] A. N. Chantis, M. van Schilfgaarde, and T. Kotani, Phys. Rev. Lett. **96**, 086405 (2006).
[6] I. D'Amico and C. A. Ullrich, Phys. Rev. B **74**, 121303(R) (2006).
[7] A. Pinczuk, S. Schmitt-Rink, G. Danan, J. P. Valladares, L. N. Pfeiffer, and K. W. West, Phys. Rev. Lett. **63**, 1633 (1989).
[8] R. D'Agosta and G. Vignale, Phys. Rev. Lett. **96**, 016405 (2006).
